# Supplementary material for: Hall effect driven by non-collinear magnetic polarons in diluted magnetic semiconductors
Source: arXiv:1801.09459 source file (2018-01-29)
Supplement: Supplementary file 1 [file suppl.pdf]

# Hall effect driven by non-collinear magnetic polarons in diluted magnetic semiconductors - Supplemental Materials

K. S. Denisov[1, 2, *] and N. S. Averkiev[1]

[1]Ioffe Institute, 194021 St.Petersburg, Russia

[2]Lappeenranta University of Technology, FI-53851 Lappeenranta, Finland

(Dated: January 29, 2018)

## APPENDIX A: WAVE-FUNCTIONS OF A 2D LOCALIZED STATE WITH SPIN-ORBIT INTERACTION

In the Supplemental Material we derive the planar wave-function $\psi_\nu(\boldsymbol{\rho})$ of a carrier (with 1/2 pseudospin $\boldsymbol{j}$) bound state in a short-range potential $V_0(\rho)$ in presence of spin-orbit interaction $H_{SO}$. The $\psi_\nu(\boldsymbol{\rho})$ satisfies:

$$\left(-\frac{\hbar^2}{2m}\nabla^2 + H_{SO} + V_0(\rho) - E_0\right)\psi_\nu(\boldsymbol{\rho}) = 0 \qquad \text{(A1)}$$

where $m$ is an in-plane effective mass, and $E_0$ is an energy of bound state counted from a subband edge in abscence of spin-orbit splitting (Fig.1). We consider only the $\boldsymbol{k}$-linear spin-orbit terms of either Rashba or Dresselhaus type, thus $H_{SO}$ reads as:

$$\begin{aligned} H^R_{SO} &= \beta^R_{SO}\left(\sigma_x k_y - \sigma_y k_x\right) \\ H^D_{SO} &= \beta^D_{SO}\left(\sigma_x k_x - \sigma_y k_y\right) \end{aligned} \qquad \text{(A2)}$$

where $\beta^{R,D}_{SO}$ is a spin-orbit coupling strength, $\boldsymbol{j} = \boldsymbol{\sigma}/2$ (the axis $x||[100], y||[010]$, $z||[001]$, QW is growned along $z$-axis). The term $H^D_{SO}$ coincides with $H^R_{SO}$ upon the replacement $k_x \leftrightarrow k_y$, so we discuss further the Rashba splitting. The general form of $\psi_\nu(\boldsymbol{\rho})$ for the lower bound Kramers pair $\nu = 1, 2$ is:

$$\psi_1(\boldsymbol{\rho}) = \begin{pmatrix} a(\rho) \\ e^{i\theta} b(\rho) \end{pmatrix}, \qquad \psi_2(\boldsymbol{\rho}) = -i\sigma_y \psi_1^*(\boldsymbol{\rho}) \qquad \text{(A3)}$$

where $\theta$ is a polar angle, the functions $a(\rho), b(\rho)$ are determined by $V_0(\rho)$. For the short-range potential with a spatial size $r_0$ much smaller than a localization length $a_B$ the wave-function outside $r_0$ are found according to the zero-radius potential method. The latter states that $\psi_\nu(\boldsymbol{\rho})$ are given by solutions of a free Hamiltonian with the energy $E_0$ of a bound level taken as a parameter. The equation for $\psi_\nu(\boldsymbol{\rho})$ then reads as

$$\begin{aligned} &\left(\frac{1}{\rho}\partial_\rho \rho \partial_\rho - \frac{1}{\rho^2}\partial_\theta - q_0^2 + H_{SO}\right)\psi_\nu(\boldsymbol{\rho}) = 0 \\ &H_{SO} = 2q_{SO}\begin{pmatrix} 0 & e^{-i\theta}\left(-\partial_\rho + \frac{i}{\rho}\partial_\theta\right) \\ e^{i\theta}\left(\partial_\rho + \frac{i}{\rho}\partial_\theta\right) & 0 \end{pmatrix} \end{aligned} \qquad \text{(A4)}$$

where $q_0^2 = 2m|E_0|/\hbar^2$, $q_{SO} = m\beta_{SO}/\hbar^2$, and we introduce the parameter $\delta_{SO} = q_{SO}/q_0$. The solutions decreasing away from center are given by a combination of modified Bessel functions of the second kind $K_0(z), K_1(z)$[4]:

$$\psi_1(\boldsymbol{\rho}) = \begin{pmatrix} c_1 K_0(q\rho) \\ c_2 e^{i\theta} K_1(q\rho) \end{pmatrix} \qquad \text{(A5)}$$

where the parameter $q$ (complex number with positive real part) and $c_{1,2}$ are determined from the secular equation:

$$\begin{pmatrix} q^2 - q_0^2 & 2qq_{SO} \\ -2qq_{SO} & q^2 - q_0^2 \end{pmatrix}\begin{pmatrix} c_1 \\ c_2 \end{pmatrix} = 0.$$

Two complex eigenvalues $q_\pm = \sqrt{q_0^2 - q_{SO}^2} \pm iq_{SO}$ correspond to two linearly independent wave-functions[1]:

$$\psi_1^\pm(\boldsymbol{\rho}) = q_\pm \begin{pmatrix} K_0(q_\pm \rho) \\ \mp i e^{i\theta} K_1(q_\pm \rho) \end{pmatrix}.$$

According to zero-potential method, the wave-function $\psi_1(\boldsymbol{\rho})$ that describes the localized state is given by the normalized combination of $\psi_1^\pm$. We write it down:

$$\psi_1(\boldsymbol{\rho}) = c_0 \begin{pmatrix} \mathrm{Re}\left[q_+ K_0(q_+ r)\right] \\ e^{i\theta}\mathrm{Im}\left[q_+ K_1(q_+ r)\right] \end{pmatrix}, \qquad \psi_2 = -i\sigma_y \psi_1^* \qquad \text{(A6)}$$

where $c_0$ is a normalization constant given by:

$$c_0 = \frac{1}{\sqrt{\pi}}\left(1 - \frac{q_+ - q_-}{2(q_+ + q_-)}\ln\frac{q_+}{q_-}\right)^{-1/2}$$

We notice that $\psi_\nu$ might also be obtained from the Fourier transformation of (A1)[2,3].

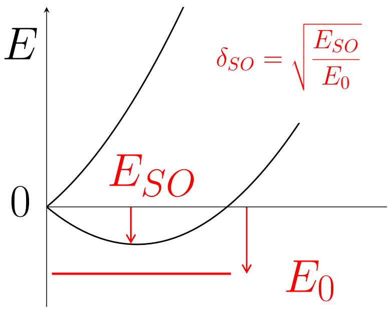


FIG. 1: Energy dispesion of free motion states and the position of a localized level $E_0$.

The wave-functions of the Dresselhaus spin-orbit splitting are obtained by the replacement $\theta \to \pi/2 - \theta$ (this corresponds to $k_x \leftrightarrow k_y$ in (A4)) in $\psi_1(\boldsymbol{\rho})$:

$$\psi_1(\boldsymbol{\rho}) = c_0 \begin{pmatrix} \mathrm{Re}\,[q_+ K_0(q_+ r)] \\ ie^{-i\theta}\mathrm{Im}\,[q_+ K_1(q_+ r)] \end{pmatrix} \qquad \psi_2 = -i\sigma_y \psi_1^* \tag{A7}$$

In the main article we denote the $\rho$-dependent part as

$$\begin{aligned} a(\rho) &= c_0 \mathrm{Re}\,[q_+ K_0(q_+ \rho)] \\ b(\rho) &= c_0 \mathrm{Im}\,[q_+ K_1(q_+ \rho)]\,. \end{aligned} \tag{A8}$$

Since $q_+ = q_0(\sqrt{1-\delta_{SO}^2} + i\delta_{SO})$ has an imaginary part, the function $a, b$ have an oscillating structure and $b \neq 0$.

## APPENDIX B: TRANSITION TO A MAGNETIC SKYRMION

In this section we consider the transition of a BMP ground state to a skyrmion (antiskyrmion) configuration at large spin-orbit couplings $\delta_{SO}$. The exchange field $\boldsymbol{B}_{ex}$ generated by the planar wave-functions $\psi_\nu$ from (A6,A7) is given by:

$$\begin{aligned} \boldsymbol{B}_{ex}^x(\boldsymbol{\rho}) &= \zeta g_{\|} a(\rho) b(\rho) \cos(\varkappa\theta + \gamma) \\ \boldsymbol{B}_{ex}^y(\boldsymbol{\rho}) &= \zeta g_{\|} a(\rho) b(\rho) \sin(\varkappa\theta + \gamma) \\ \boldsymbol{B}_{ex}^z(\rho) &= \zeta g_z \frac{(-1)^\nu}{2} \left(b^2(\rho) - a^2(\rho)\right) \end{aligned} \tag{B1}$$

where $\zeta = (\alpha_{ex}/g_0\mu_B d_{QW})$, $\varkappa = \pm 1$ for Rashba and Dresselhaus terms, $\gamma$ is an initial phase. We consider the case when the external magnetic field $\boldsymbol{B}_0 || z$ is directed along the QW growth axis $z$. Let us calculate the Mn spins $\boldsymbol{I}(\boldsymbol{\rho})$ energy difference in two cases: when only an external field $\boldsymbol{B}_0$ is applied, and when there is also an exchange field $\boldsymbol{B}_{ex}$ due to a localized carrier. The orientation of Mn for these two situation at the limit $T \to 0$ is parallel either to $\boldsymbol{B}_0$ or to the total field $\boldsymbol{B}_{tot}^\nu(\boldsymbol{\rho}) = \boldsymbol{B}_0 + \boldsymbol{B}_{ex}^\nu(\boldsymbol{\rho})$. The energy difference of these configurations is given by:

$$\Delta E_p^\nu = (g_0\mu_B I) n_0 \int d\boldsymbol{\rho}\,(B_0 - B_{tot}^\nu(\boldsymbol{\rho})) \tag{B2}$$

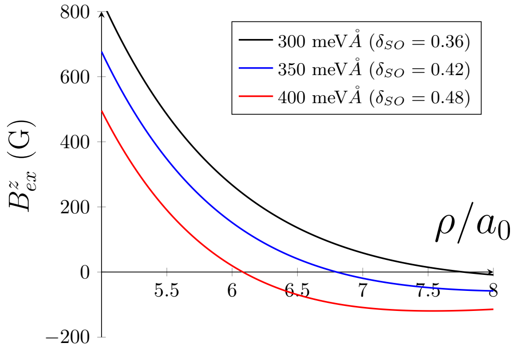


FIG. 2: The dependence of $\boldsymbol{B}_{ex}^z(\rho)$ on distance from polaron center $\rho$ for different spin-orbit couplings $\beta_{SO} = 300, 350, 400$ meV$\mathring{A}$. The spatial coordinates are given in lattice constant $a_0$.

where $n_0 = x_{Mn} N_0 d_{QW}$ is Mn 2D density, $N_0$ is a number of cations per unit cell, $x_{Mn}$ the fraction of Mn, $d_{QW}$ is QW thickness; we use a meanfield approximation assuming that there is a big number of magnetic impurities inside a BMP core. The ground state of BMP has lower $\Delta E_p$. The gain in energy occurs when the $z$-component of $\boldsymbol{B}_{ex}$ is so-aligned with $\boldsymbol{B}_0$ for the majority of spin inside BMP. Let us consider the effect of spin-orbit interaction on this issue.

In Fig.2 we show the dependence of the z-component of exchange field $\boldsymbol{B}_{ex}^z(\rho)$ given by (B1) on a distance from polaron center at different $\delta_{SO}$. For small $\delta_{SO}$ the sign of $\boldsymbol{B}_{ex}^z(\rho)$ does not change inside BMP ($\delta_{SO} = 0.36$ in Fig.2). In this case the more favorable configuration (ground state) obviously has $\eta = 1$ (so-aligned). At larger spin-orbit coupling ($\delta_{SO} = 0.42, 0.48$ in Fig.2) the sign of $\boldsymbol{B}_{ex}^z(\rho)$ on the periphery and in the vicinity of polaron center is opposite. When the magnitude of the external field $B_0$ is of the same order as the typical values of $B_{ex}^z$ in the periphery region with opposite sign, it turns out that it is more favorable to orient periphery spins along $\boldsymbol{B}_0$, while the spins next to the center will be automatically directed anti-parallel (ground state corresponds to $\eta = -1$).

In Fig.3 we show the dependence of $\Delta E_p^\nu$ on $B_0$ for $\delta_{SO} = 0.48$ ($\beta_{SO} = 400$ meV$\mathring{A}$). At small $B_0 \leq 600$ G the skyrmion configuration has lower energy. The typical energy distance between two states is $\sim 0.5$ meV. The larger ($B_0 \geq 600$ G ) external fields suppress the weak periphery exchange field, so there is a transition to $\eta = 1$ ground state. At small $\delta_{SO}$ the $\eta = 1$ configuration is always more favorable. Let us mention that the observation of the "topological transition" requires ultra-low temperatures. The critical temperature cannot exceed the magnitude of the exchange field on the periphery, which according to Fig.2 is $\leq 200$ G. The corresponding temperature $T \leq 100$ mK.

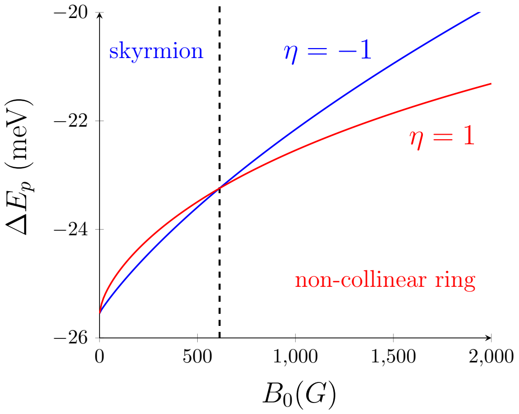


FIG. 3: BMP energy for $\eta = \pm 1$. At $B_0 \leq 600$ G the skyrmion (antiskyrmion) configuration $\eta = -1$ has lower energy.

---

* Electronic address: `denisokonstantin@gmail.com`


[1] A. V. Chaplik and L. I. Magarill, Phys. Rev. Lett. **96**, 126402 (2006).

[2] K. S. Denisov and N. S. Averkiev, JETP Letters **99**, 400 (2014).

[3] I. V. Rozhansky, M. B. Lifshits, S. A. Tarasenko, and N. S. Averkiev, Phys. Rev. B **80**, 085314 (2009).


[4] We use the recurrent relations $(\partial_r + 1/r)\, K_1(qr) = -qK_0(qr)$, and $\partial_r K_0(qr) = -qK_1(qr)$.
